# Supplementary material for: Theory of Fractionally-magnetized Quantum Ferromagnet
Source: arXiv:2308.15372 ancillary file (2023-08-29)
Supplement: Supplementary file 1 [file supplements.pdf]

# Supplement

This is a supplement for the paper
"Theory of Fractionally-magnetized Quantum Ferromagnet"
by I. Maruyama and S. Miyahara. The supplement is organized as follows: section (S.1) provides a demonstration of three Hamiltonians and coefficients Jij in the paper, and section (S.2) provides a demonstration and a proof of rigorous eigenstate correspondence. The demonstration and theorem proving for small system-size will make the points of the paper more convincing. The definition code of Mathematica with basic explanation will help general readers catch up the general statements in the paper. In addition, user's trial of the demonstration with arbitrary parameters will support his/her further studies.

To evaluate all demonstrations, push CTRL+A and SHIFT+ENTER in Mathematica notebook. We use Mathematica 13.0.1 for win 64-bit.

In[1]:=
```
Clear["Global`*"];
$Version
```

Out[2]=
```
13.0.1 for Microsoft Windows (64-bit) (January 28, 2022)
```

# S. 1: Hamiltonian Hα, Hr, and Hc

The spin-S BLBQ Hamiltonian with one-parameter $\alpha$ is
Hα^(S) = cosα Σ_i Si · Si+1 + sinα Σ_i (Si · Si+1)^2 ,  Eq.(1) in the paper,
which is also written in the form of the spin-projection Hamiltonian Σijs Jij(s) Pij(s) via Eq.(4) with the coefficient Jij(s) as a function of $\alpha$;
Jij(s)= cosα q(s) + sin α q(s)^2,  in the next paragraph below Eq(5),
with q(s)=s(s+1)/2-S(S+1), defined below Eq.(4). The high-symmetric points αr and αc are defined in Eq.(2) and Eq.(3), respectively.

In[3]:=
```
αr[S_]:=If[S≤3/2,0,Pi]-ArcTan[1/(2S(S-2)+1)]; (* Eq.(2)*)
αc[S_]:=Pi-ArcTan[1/(2S(S-1))]; (* Eq.(3)*)
q[s_,S_]:=s (s+1)/2-S(S+1); (* below Eq.(4) *)
Jij[s_,S_,a_]:=Cos[a]q[s,S]+Sin[a]q[s,S]^2;
```

To show the high-symmetric points, we plot Jij(s) as a function $\alpha$ for S=3/2, and S=2.

In[4]:=
```
v[t_,b_,s_:1/2]:=Subsuperscript[t,b,"("<>ToString[s,InputForm]<>")"];
pl[S_]:=Block[{f,p,α,J,ij},
f=Table[Jij[s,S,α],{s,0,2S}];
p={Join[{{αr[S],v[α,"r",S]},{αc[S],v[α,"c",S]}},Range[4]/2 π],All};
Plot[f,{α,0,2π},PlotLabel→"S="<>ToString[S,InputForm],
PlotLegends→Map[#⟦1⟧==#⟦2⟧&,Transpose[{Table[v[J,ij,s],{s,0,2S}],f}]],
AxesLabel→{α,v[J,ij,s]},Ticks→p,GridLines→Automatic]];
{pl[3/2],pl[2]}//Column (* one can add pl[5/2], pl[3], and so on *)
```

Out[6]=

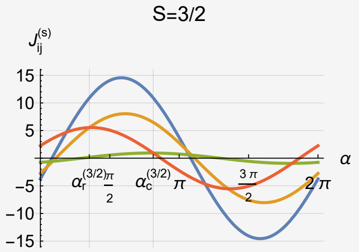


$J_{ij}^{(0)} = \frac{225 \sin(\alpha)}{16} - \frac{15 \cos(\alpha)}{4}$

$J_{ij}^{(1)} = \frac{121 \sin(\alpha)}{16} - \frac{11 \cos(\alpha)}{4}$

$J_{ij}^{(2)} = \frac{9 \sin(\alpha)}{16} - \frac{3 \cos(\alpha)}{4}$

$J_{ij}^{(3)} = \frac{81 \sin(\alpha)}{16} + \frac{9 \cos(\alpha)}{4}$

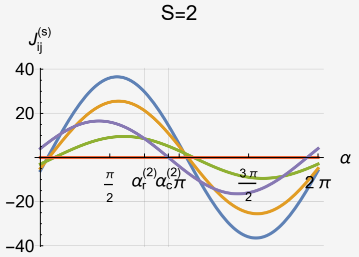


$J_{ij}^{(0)} = 36 \sin(\alpha) - 6 \cos(\alpha)$

$J_{ij}^{(1)} = 25 \sin(\alpha) - 5 \cos(\alpha)$

$J_{ij}^{(2)} = 9 \sin(\alpha) - 3 \cos(\alpha)$

$J_{ij}^{(3)} = 0$

$J_{ij}^{(4)} = 16 \sin(\alpha) + 4 \cos(\alpha)$

The above figures show intersecting points of coefficients Jij(s) at the high-symmetric points αr and αc. As results, the condition of the rigorous-eigenstate-correspondence Hamiltonian Hr in Eq.(5), Jij(2S)=Jij(2S-2) and that of the critical Hamiltonian Hc in Eq.(6), Jij(2S)=Jij(2S-1)<Jij(s), are satisfied.

The BLBQ Hamiltonian H_{α}^(S) at αr is rewritten with the projection operators as follows.

In[7]:=
```
HαinP[S_,α_]:=Sum[Jij[s,S,α]×v[P,ij,s],{s,0,2S}]; (* Hamiltonian Hα written in P *)
Heq[S_,r_,a_]:=TraditionalForm[v[H,r,S]==v[H,a,S] == Subscript[Σ,ij]×HαinP[S,a]];
Table[Heq[S,r,αr[S]],{S,1,3,1/2}]//Column (* from S=1 to S=3 *)
```

Out[8]=

$$H_r^{(1)} = H_{\frac{\pi}{4}}^{(1)} = \Sigma_{ij} \left( \sqrt{2}\, P_{ij}^{(0)} + \sqrt{2}\, P_{ij}^{(2)} \right)$$

$$H_r^{(3/2)} = H_{\tan^{-1}(2)}^{(3/2)} = \Sigma_{ij} \left( \frac{39}{8} \sqrt{5}\, P_{ij}^{(0)} + \frac{99\, P_{ij}^{(1)}}{8 \sqrt{5}} + \frac{3\, P_{ij}^{(2)}}{8 \sqrt{5}} + \frac{99\, P_{ij}^{(3)}}{8 \sqrt{5}} \right)$$

$$H_r^{(2)} = H_{\frac{3\pi}{4}}^{(2)} = \Sigma_{ij} \left( 21 \sqrt{2}\, P_{ij}^{(0)} + 15 \sqrt{2}\, P_{ij}^{(1)} + 6 \sqrt{2}\, P_{ij}^{(2)} + 6 \sqrt{2}\, P_{ij}^{(4)} \right)$$

$$H_r^{(5/2)} = H_{\pi-\tan^{-1}\left(\frac{2}{7}\right)}^{(5/2)} = \Sigma_{ij} \left( \frac{1715\, P_{ij}^{(0)}}{8 \sqrt{53}} + \frac{1395\, P_{ij}^{(1)}}{8 \sqrt{53}} + \frac{851\, P_{ij}^{(2)}}{8 \sqrt{53}} + \frac{275\, P_{ij}^{(3)}}{8 \sqrt{53}} - \frac{45\, P_{ij}^{(4)}}{8 \sqrt{53}} + \frac{275\, P_{ij}^{(5)}}{8 \sqrt{53}} \right)$$

$$H_r^{(3)} = H_{\pi-\tan^{-1}\left(\frac{1}{7}\right)}^{(3)} = \Sigma_{ij} \left( \frac{114}{5} \sqrt{2}\, P_{ij}^{(0)} + \frac{99}{5} \sqrt{2}\, P_{ij}^{(1)} + \frac{72}{5} \sqrt{2}\, P_{ij}^{(2)} + \frac{39}{5} \sqrt{2}\, P_{ij}^{(3)} + \frac{9}{5} \sqrt{2}\, P_{ij}^{(4)} - \frac{6}{5} \sqrt{2}\, P_{ij}^{(5)} + \frac{9}{5} \sqrt{2}\, P_{ij}^{(6)} \right)$$

The results represent the Eq.(5) with certain parameters. For αr + π, one can modify above as "Heq[S,c,αr[S]+Pi]". Also, the BLBQ Hamiltonian H_{α}^(S) at αc is rewritten with the projection operators as follows.

In[9]:=
```
Table[Heq[S,c,αc[S]],{S,3/2,3,1/2}]//Column (* from S=3/2 to S=3 *)
```

Out[9]=

$$H_c^{(3/2)} = H^{(3/2)}_{\pi-\tan^{-1}\left(\frac{2}{3}\right)} = \Sigma_{ij}\left(\frac{315\,P_{ij}^{(0)}}{8\sqrt{13}} + \frac{187\,P_{ij}^{(1)}}{8\sqrt{13}} + \frac{27\,P_{ij}^{(2)}}{8\sqrt{13}} + \frac{27\,P_{ij}^{(3)}}{8\sqrt{13}}\right)$$

$$H_c^{(2)} = H^{(2)}_{\pi-\tan^{-1}\left(\frac{1}{4}\right)} = \Sigma_{ij}\left(\frac{60\,P_{ij}^{(0)}}{\sqrt{17}} + \frac{45\,P_{ij}^{(1)}}{\sqrt{17}} + \frac{21\,P_{ij}^{(2)}}{\sqrt{17}}\right)$$

$$H_c^{(5/2)} = H^{(5/2)}_{\pi-\tan^{-1}\left(\frac{2}{15}\right)} = \Sigma_{ij}\left(\frac{2275\,P_{ij}^{(0)}}{8\sqrt{229}} + \frac{1891\,P_{ij}^{(1)}}{8\sqrt{229}} + \frac{1219\,P_{ij}^{(2)}}{8\sqrt{229}} + \frac{451\,P_{ij}^{(3)}}{8\sqrt{229}} - \frac{125\,P_{ij}^{(4)}}{8\sqrt{229}} - \frac{125\,P_{ij}^{(5)}}{8\sqrt{229}}\right)$$

$$H_c^{(3)} = H^{(3)}_{\pi-\tan^{-1}\left(\frac{1}{12}\right)} = \Sigma_{ij}\left(\frac{288\,P_{ij}^{(0)}}{\sqrt{145}} + \frac{253\,P_{ij}^{(1)}}{\sqrt{145}} + \frac{189\,P_{ij}^{(2)}}{\sqrt{145}} + \frac{108\,P_{ij}^{(3)}}{\sqrt{145}} + \frac{28\,P_{ij}^{(4)}}{\sqrt{145}} - \frac{27\,P_{ij}^{(5)}}{\sqrt{145}} - \frac{27\,P_{ij}^{(6)}}{\sqrt{145}}\right)$$

As shown above, the condition Jij(2S)=Jij(2S-1)<Jij(s) is satisfied. Note that $\alpha$c is not defined at S=1 but one can get $\alpha$c -> Pi/2 in the limit S-> 1+0. Then, one can get the spin-1 Hamiltonian with the relation Jij(2)=Jij(1)=1 < Jij(0)=4 as follows.

In[10]:=
```
Heq[1,c,Limit[αc[S],S→1,Direction→-1]]
```

Out[10]//TraditionalForm=

$$H_c^{(1)} = H^{(1)}_{\frac{\pi}{2}} = \Sigma_{ij}\left(4\,P_{ij}^{(0)} + P_{ij}^{(1)} + P_{ij}^{(2)}\right)$$

If we use the identity Pij(0)+Pij(1)+Pij(2)=1, then H$\alpha$c^(S=1) becomes 3Pij(0) + constant. This is nothing but Hc^(S=1) at the phase-boundary between ferro. and trimer phase in S=1 BLBQ chain as shown in Fig. 1 of the paper.

# S. 2: Rigorous eigenstate correspondence

The proof of rigorous eigenstate correspondence between spin-S Hamiltonian Hr^(S) and spin-1/2 Hamiltonian H^(1/2) is based on

Hr^(S) ℂ= ℂ H^(1/2) , (S0)

which is written in the note[30] of the paper. Let $|\psi\rangle$ be an eigenstate of H^(1/2) with an eigen energy $\epsilon$, that is, H^(1/2)$|\psi\rangle=\epsilon|\psi\rangle$. Then, one can show a state |Ψ0⟩=ℂ $|\psi\rangle$ is an eigenstate of Hr^(S) with the same eigen energy as

Hr^(S) |Ψ0⟩ = Hr^(S) ℂ $|\psi\rangle$ = ℂ H^(1/2) $|\psi\rangle$ = ℂ $\epsilon\,|\psi\rangle = \epsilon\,$|Ψ0⟩.

In the second equation, Eq.(S0) was used. In this sense, Eq.(S0) is a key of the proof, which is the target of this section. Eq.(S0) is defined as a variable Eq[S0] in Mathematica as follows:

In[11]:=
```
Eq[S0]:=Hr . ℂ[S,L]==ℂ[S,L] . Honehalf  (* note[30] *)
```

Here, "Honehalf" is the spin-1/2 Hamiltonian H^(1/2). The definition of Hr, ℂ, and Honehalf will be given in S.2-1 and we will demonstrate that Eq.(S0) is satisfied for given (small) system-size L and spin S. The proofs for general L and general S are given in S.2-2 and 2-3, respectively. Finally, the proof of Eq.(S0) for general L and S will be summarized in S.2-4.

## S. 2-1 Demo. of Eq.(S0) for given L, S

To demonstrate that Eq.(S0) is satisfied for given system-size L and spin-S, we prepare operators (matrices);

SdS[i,j,L,S] as the Heisenberg interaction term Si·Sj=Sxi Sxj+Syi Syj+Szi Szj,

P[s,S,i,j,L] as the spin-projection Pij^(s) for s=0,1,...,2S,
ℂ[S,L] as the intertwiner C defined below Eq.(5),
Hr as the spin-projection Hamiltonian Hr^(S) in Eq.(5),
Honehalf as corresponding spin-1/2 Heisenberg Hamiltonian H^(1/2) defined below Eq.(5),
as follows. One can skip the detail.

In[12]:=
```
id[m_]:=SparseArray[{{i_,i_}→1},Dimensions[m]];
op2[m1_,m2_,i1_:1,i2_:2,l_:2]:=opa[l,id[m1],<|i1→m1,i2→m2|>];
op1[m_,i_,l_]:=opa[l,id[m],<|i→m|>];
opa[l_,id_,a_:<||>]:=KroneckerProduct@@Table[Lookup[a,Mod[i,l,1],id],{i,1,l}];
Sop[S_]:=Block[{m,Sz,Sp,Sm,Sy,Sx,i},
m[i_]:=-(Mod[i,2S+1,1]-S-1);
Sz:=SparseArray[{i_,i_}→m[i],{2S+1,2S+1}];
Sp:=SparseArray[Table[{i-1,i}→ Sqrt[(S-m[i])(S+m[i]+1)],{i,2,2S+1}],{2S+1,2S+1}];
Sm:=ConjugateTranspose[Sp];
Sx:=(Sp+Sm)/2;
Sy:=(Sp-Sm)/(2I);
{Sx,Sy,Sz,id[Sz],Sp,Sm}
];
SdS[i_:1,j_:2,l_:2,s_:1/2]:=Sum[op2[o,o,i,j,l],{o,Sop[s]〚1;;3〛}];
P0[sds_,s_,S_]:=Dot@@Table[(sds-q[m,S]*id[sds])/(q[s,S]-q[m,S]),
{m,Select[Range[0,2S],#≠s&]}]; (* Eq.(4) *)
P[s_,S_:1/2,i_:1,j_:2,l_:2]:=P0[SdS[i,j,l,S],s,S];
ket[m_,s_:1/2]:=SparseArray[{(s-m)+1}→1,2s+1];
diad[v1_,v2_]:=ConjugateTranspose[{v1}] . {v2};
ℂi[S_]:=diad[ket[S,S],ket[1/2]]+diad[ket[S-1,S],ket[-1/2]]; (* below Eq.(5) *)
ℂ[S_,L_:2]:=opa[L,ℂi[S]];
defH[S_,L_]:=Block[{},Clear[J];
J[i_,j_,2S-2]:=J[i,j,2S];(* condition for Hr *)
J[i_,i_,s_]:=0;(* Jii=0 because we don't consider Pii *)
Hr:=Sum[J[i,j,s]*P[s,S,i,j,L],{i,1,L},{j,1,L},{s,0,2S}];
(* Hr is Hr^(S) in Eq.(5) *)
Honehalf:=Sum[(J[i,j,2S]-J[i,j,2S-1])*SdS[i,j,L]+
(3 J[i,j,2S]+J[i,j,2S-1])/4*id[SdS[i,j,L]],{i,1,L},{j,1,L}];
(* Honehalf is H^(1/2) defined below Eq.(5) *)];
```

Here we are ready to evaluate Eq.(S0): Hr^(S) ℂ= ℂ H^(1/2) .

In[23]:=
```
L=4;(* you can modify systemsize L*)
S=3/2;(* you can modify spin-S*)
defH[S,L];(* define Hr and Honehalf *)
Eq[S0]//FullSimplify
```

Out[23]=
```
True
```

The return value "True" means Eq.(S0) is valid for given system-size L=4 and spin S=3/2. You can modify L and S and check the validity for arbitrary values. Note that the corresponding Hamiltonian H^(1/2) has general coefficients as variable. For example, (1,1)-element of H^(1/2), (Honehalf)_{1,1}, has coefficient J(i=1,j=2,s=3),..., and so-on;

In[24]:=
```
Honehalf⟦1,1⟧//FullSimplify//TraditionalForm
(* (1,1)-element *)
```

Out[24]//TraditionalForm=

$$J(1,2,3)+J(1,3,3)+J(1,4,3)+J(2,1,3)+J(2,3,3)+ J(2,4,3)+J(3,1,3)+J(3,2,3)+J(3,4,3)+J(4,1,3)+J(4,2,3)+J(4,3,3)$$

For more direct demonstration of the rigorous eigenstate correspondence, let us calculate eigensystem in the case of random coefficients Jij(s) [s=2S and 2S-1] for system-size L=4 and S=3/2.

In[25]:=
```
L=4;S=3/2;
defH[S,L];(* clear J, define Hr and Honehalf *)
(* Here we test random Hamiltonian. You can use more traditional Hamiltonian. *)
rnd=Table[RandomInteger[L^2],{i,1,L},{j,1,L},{k,1,2}];
J[i_,j_,2S]:=If[i≠j,rnd⟦i,j,1⟧,0];
J[i_,j_,2S-1]:=If[i≠j,rnd⟦i,j,2⟧,0];
```

Eigenvalues $\epsilon$ and eigenvectors $\psi$ for corresponding spin-1/2 system "Honehalf" can be calculated by the function Eigensystem and checked by a function eygensystemCheck.

In[29]:=
```
{ϵ,ψ}=Eigensystem[Honehalf];
eigensystemCheck[H_,e_,p_]:=And@@Table[Norm[FullSimplify[
H . p⟦i⟧-e⟦i⟧*p⟦i⟧]]==0,{i,1,Length[e]}];
eigensystemCheck[Honehalf,ϵ,ψ]
```

Out[31]= True

The return value "True" means the eigensystem ($\epsilon$,$\psi$) are really eigensystem of Honehalf.

In addition, let us demonstrate the validity of the sentence "for any eigenstate $|\psi\rangle$ of H^(1/2), corresponding eigenstate of Hr^(S) are rigorously written as $|\Psi 0\rangle=\mathbb{C}\,|\psi\rangle$" below Eq.(5) in the paper. A subset of eigenvalues E and eigenvectors Ψ for original spin-S Hamiltonian Hr can be obtained from the eigensystem ($\epsilon$,$\psi$) for "Honehalf" as

$|\Psi 0\rangle=\mathbb{C}\,|\psi\rangle$, below Eq.(5) in the paper,

E=$\epsilon$,

for any eigenvector $\psi$ for Honehalf. Spin-S eigensystem ($\epsilon$,Ψ0) can be checked by the function eigensystemCheck.

In[32]:=
```
Ψ0=Table[ℂ[S,L] . p,{p,ψ}];
E=ϵ;
eigensystemCheck[Hr,E,Ψ0]
```

Out[34]= True

The return value "True" means that given (E,Ψ0) is a subset of the eigensystem of Hr. It should be emphasized that (E,Ψ0) is not calculated from Hr but obtained from ($\epsilon$,$\psi$) of Honehalf via ℂ. One can check Honehalf, Hr, $\psi$, and Ψ0 as follows.

In[35]:=
```
mf[m_]:=TraditionalForm[FullSimplify[Normal[m]]];
Honehalf//mf (* 2^L dim matrix with random integer coeff. *)
```

Out[36]//TraditionalForm=

$$\begin{pmatrix}
88 & 0 & 0 & 0 & 0 & 0 & 0 & 0 & 0 & 0 & 0 & 0 & 0 & 0 & 0 & 0 \\
0 & 87 & -2 & 0 & 4 & 0 & 0 & 0 & -1 & 0 & 0 & 0 & 0 & 0 & 0 & 0 \\
0 & -2 & 95 & 0 & -2 & 0 & 0 & 0 & -3 & 0 & 0 & 0 & 0 & 0 & 0 & 0 \\
0 & 0 & 0 & 90 & 0 & -2 & 4 & 0 & 0 & -3 & -1 & 0 & 0 & 0 & 0 & 0 \\
0 & 4 & -2 & 0 & \frac{179}{2} & 0 & 0 & 0 & -\frac{7}{2} & 0 & 0 & 0 & 0 & 0 & 0 & 0 \\
0 & 0 & 0 & -2 & 0 & \frac{193}{2} & -2 & 0 & 0 & -\frac{7}{2} & 0 & 0 & -1 & 0 & 0 & 0 \\
0 & 0 & 0 & 4 & 0 & -2 & \frac{185}{2} & 0 & 0 & 0 & -\frac{7}{2} & 0 & -3 & 0 & 0 & 0 \\
0 & 0 & 0 & 0 & 0 & 0 & 0 & \frac{191}{2} & 0 & 0 & 0 & -\frac{7}{2} & 0 & -3 & -1 & 0 \\
0 & -1 & -3 & 0 & -\frac{7}{2} & 0 & 0 & 0 & \frac{191}{2} & 0 & 0 & 0 & 0 & 0 & 0 & 0 \\
0 & 0 & 0 & -3 & 0 & -\frac{7}{2} & 0 & 0 & 0 & \frac{185}{2} & -2 & 0 & 4 & 0 & 0 & 0 \\
0 & 0 & 0 & -1 & 0 & 0 & -\frac{7}{2} & 0 & 0 & -2 & \frac{193}{2} & 0 & -2 & 0 & 0 & 0 \\
0 & 0 & 0 & 0 & 0 & 0 & 0 & -\frac{7}{2} & 0 & 0 & 0 & \frac{179}{2} & 0 & -2 & 4 & 0 \\
0 & 0 & 0 & 0 & 0 & -1 & -3 & 0 & 0 & 4 & -2 & 0 & 90 & 0 & 0 & 0 \\
0 & 0 & 0 & 0 & 0 & 0 & 0 & -3 & 0 & 0 & 0 & -2 & 0 & 95 & -2 & 0 \\
0 & 0 & 0 & 0 & 0 & 0 & 0 & -1 & 0 & 0 & 0 & 4 & 0 & -2 & 87 & 0 \\
0 & 0 & 0 & 0 & 0 & 0 & 0 & 0 & 0 & 0 & 0 & 0 & 0 & 0 & 0 & 88
\end{pmatrix}$$

In[37]:=
```
nth=1;(* one can modify *)
ψ[[nth]]//FullSimplify (* nth eigenvector of Honehalf *)
```

Out[37]=

$$\left\{0, 0, 0, 1, 0, \frac{1}{8}\left(-13-\sqrt{129}\right), \frac{1}{8}\left(5+\sqrt{129}\right), 0, 0, \frac{1}{8}\left(5+\sqrt{129}\right), \frac{1}{8}\left(-13-\sqrt{129}\right), 0, 1, 0, 0, 0\right\}$$

One can plot the elements of (2S+1)^L -dimensional matrix Hr^(S), instead of the command "Hr//mf" which is too large to show below.

In[38]:=
```
Hr//MatrixPlot  (* (2S+1)^L dim. *)
```

Out[38]=

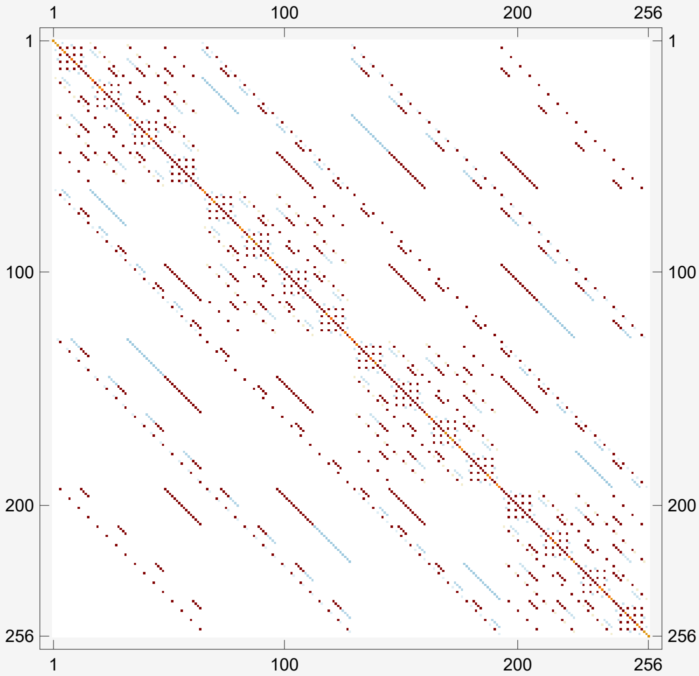


In[39]:=
```
Ψ0⟦nth⟧//FullSimplify (* nth eigenvector of Hr *)
```

Out[39]=

{0, 0, 0, 0, 0, 1, 0, 0, 0, 0, 0, 0, 0, 0, 0, 0, $\frac{1}{8}\left(-13-\sqrt{129}\right)$, 0, 0, $\frac{1}{8}\left(5+\sqrt{129}\right)$, 0, 0,
0, 0, 0, 0, 0, 0, 0, 0, 0, 0, 0, 0, 0, 0, 0, 0, 0, 0, 0, 0, 0, 0, 0, 0, 0, 0, 0, 0, 0, 0, 0,
0, 0, 0, 0, 0, 0, 0, 0, 0, 0, 0, $\frac{1}{8}\left(5+\sqrt{129}\right)$, 0, 0, $\frac{1}{8}\left(-13-\sqrt{129}\right)$, 0, 0, 0, 0, 0, 0,
0, 0, 0, 0, 0, 1, 0, 0, 0, 0, 0, 0, 0, 0, 0, 0, 0, 0, 0, 0, 0, 0, 0, 0, 0, 0, 0, 0, 0, 0, 0,
0, 0, 0, 0, 0, 0, 0, 0, 0, 0, 0, 0, 0, 0, 0, 0, 0, 0, 0, 0, 0, 0, 0, 0, 0, 0, 0, 0, 0, 0,
0, 0, 0, 0, 0, 0, 0, 0, 0, 0, 0, 0, 0, 0, 0, 0, 0, 0, 0, 0, 0, 0, 0, 0, 0, 0, 0, 0, 0, 0,
0, 0, 0, 0, 0, 0, 0, 0, 0, 0, 0, 0, 0, 0, 0, 0, 0, 0, 0, 0, 0, 0, 0, 0, 0, 0, 0, 0, 0, 0,
0, 0, 0, 0, 0, 0, 0, 0, 0, 0, 0, 0, 0, 0, 0, 0, 0, 0, 0, 0, 0, 0, 0, 0, 0, 0, 0, 0, 0, 0,
0, 0, 0, 0, 0, 0, 0, 0, 0, 0, 0, 0, 0, 0, 0, 0, 0, 0, 0, 0, 0, 0, 0, 0, 0, 0, 0, 0, 0, 0}

In[40]:=
```
Hr . Ψ0⟦nth⟧-E⟦nth⟧*Ψ0⟦nth⟧//FullSimplify
(* check eigenequation for nth eigenvector*)
```

Out[40]=

```
{0, 0, 0, 0, 0, 0, 0, 0, 0, 0, 0, 0, 0, 0, 0, 0, 0, 0, 0, 0, 0, 0, 0, 0, 0, 0, 0, 0, 0,
 0, 0, 0, 0, 0, 0, 0, 0, 0, 0, 0, 0, 0, 0, 0, 0, 0, 0, 0, 0, 0, 0, 0, 0, 0, 0, 0, 0, 0,
 0, 0, 0, 0, 0, 0, 0, 0, 0, 0, 0, 0, 0, 0, 0, 0, 0, 0, 0, 0, 0, 0, 0, 0, 0, 0, 0, 0, 0,
 0, 0, 0, 0, 0, 0, 0, 0, 0, 0, 0, 0, 0, 0, 0, 0, 0, 0, 0, 0, 0, 0, 0, 0, 0, 0, 0, 0, 0,
 0, 0, 0, 0, 0, 0, 0, 0, 0, 0, 0, 0, 0, 0, 0, 0, 0, 0, 0, 0, 0, 0, 0, 0, 0, 0, 0, 0,
 0, 0, 0, 0, 0, 0, 0, 0, 0, 0, 0, 0, 0, 0, 0, 0, 0, 0, 0, 0, 0, 0, 0, 0, 0, 0, 0, 0,
 0, 0, 0, 0, 0, 0, 0, 0, 0, 0, 0, 0, 0, 0, 0, 0, 0, 0, 0, 0, 0, 0, 0, 0, 0, 0, 0, 0,
 0, 0, 0, 0, 0, 0, 0, 0, 0, 0, 0, 0, 0, 0, 0, 0, 0, 0, 0, 0, 0, 0, 0, 0, 0, 0, 0, 0,
 0, 0, 0, 0, 0, 0, 0, 0, 0, 0, 0, 0, 0, 0, 0, 0, 0, 0, 0, 0, 0, 0, 0, 0, 0, 0, 0, 0}
```

The return value, (2S-1)^L dimensional zero vector, means Hr Ψ0_nth = E_nth * Ψ0_nth. This is valid for any random coefficients Jij(s). Here, it should be noted that the (2S-1)^L dimensional

matrix Hr includes not only pure numbers but also formulae with unset coefficients J[i,j,s] (0<= s < 2S-2), while the 2^L dimensional matrix Honehalf includes only pure numbers.  As will be shown in S.2-2, eigenstates Ψ0 are independent on the unset  coefficients Jij(s) in Hr. For example, first 3 elements of Hr that a term J[1,2, 2S-3=0 ] are shown below.

In[41]:=
```
Select[ArrayRules[Hr],(D[#⟦2⟧,J[1,2,2S-3]]≠0)&]⟦;;3⟧//Column
```

Out[41]=

$\{49, 49\} \to \frac{305}{4} + \frac{1}{4} J[1, 2, 0] + \frac{1}{4} J[2, 1, 0] + \frac{1}{4} J[2, 3, 0] + \frac{1}{4} J[2, 4, 0] + \frac{1}{4} J[3, 2, 0] + \frac{1}{4} J[4, 2, 0]$

$\{49, 97\} \to \frac{9}{2} - \frac{1}{4} J[1, 2, 0] - \frac{1}{4} J[2, 1, 0]$

$\{49, 145\} \to -\frac{9}{2} + \frac{1}{4} J[1, 2, 0] + \frac{1}{4} J[2, 1, 0]$

Although the command "Eigensystem[Hr]" that returns eigensystem of a given matrix Hr is hard for Mathematica due to the unset coefficients,  it  is easily shown that the eigenvectors obtained through |Ψ0⟩=ℂ |ψ⟩ are eigenvectors of Hr.

## S . 2 - 2 Proof for general L

Since Hr^(S) is written by Pij(2S)+Pij(2S-2),  Pij(2S-1), and the others Pij(s), (s<=2S-3), the proof of Eq.(S0) is divided into proofs of three equations;

[ Pij(2S) + Pij(2S-2) ] ℂ = ℂ pij(1),       (S1)

Pij(2S-1)  ℂ       = ℂ pij(0),       (S2)

Pij(s)  ℂ       = 0,  (s<=2S-3) ,       (S3)

where pij(s) is  spin-projection for S=1/2.  These equations can be checked as follows for i=1, i=2, system-size L=4, and spin S=3/2.

In[42]:=
```
i=1;j=2;L=4;S=3/2; (* one can modify the site i,j, system-size L, spin S *)
Eq[S1]:=(P[2S,S,i,j,L]+P[2S-2,S,i,j,L]) . ℂ[S,L]==ℂ[S,L] . P[1,1/2,i,j,L];
Eq[S2]:=P[2S-1,S,i,j,L] . ℂ[S,L]==ℂ[S,L] . P[0,1/2,i,j,L];
(* pij(1) is P[1,1/2,i,j,L] and pij(0) is P[0,1/2,i,j,L] *)
zeroMatrixQ[m_]:=And@@((#==0)&/@Flatten[m,1]);
Eq[S3]:=Table[zeroMatrixQ[P[s,S,i,j,L] . ℂ[S,L]],{s,0,2S-3}];
And@@Flatten[{Eq[S1],Eq[S2],Eq[S3]}]
```

Out[46]= True

Due to Eq.(S3), terms Jij(s) Pij(s) (s<=2S-3) in Hr^(S) have no contribution to Eq.(S0).  This is the reason why parts of Hr's eigenstates |Ψ0⟩=ℂ |ψ⟩ are determined independently of unset coefficients Jij in Hr^(S) in S.2-1.  Nonzero contribution comes from Jij(2S) ( Pij(2S)+Pij(2S-2) ) + Jij(2S-1) Pij(2S-1), satisfying Hr's limitation  Jij(2S)=Jij(2S-2).  Due to Eq.(S1) and (S2), there is the operator correspondence:

Pij(2S)+Pij(2S-2)   <---->   pij(1) ,

Pij(2S-1)       <---->   pij(0) ,

where pij(1) is triplet projection and pij(0) is singlet projection of spin-1/2 model.  In short, term Jij(2S) ( Pij(2S)+Pij(2S-2)  ) + Jij(2S-1) Pij(2S-1)  in Hrℂ  corresponds to Jij(2S)pij(1) + Jij(2S-1)pij(0) in spin-1/2 model:

Jij(2S) ( Pij(2S)+Pij(2S-2)  ) + Jij(2S-1) Pij(2S-1)  <---->  Jij(2S)pij(1) + Jij(2S-1)pij(0) .

The right hand side is written by spin-1/2 Heisenberg term as

Jij(2S)pij(1) + Jij(2S-1)pij(0)= ( Jij(2S)-Jij(2S-1) )s_i · s_j + (3 Jij(2S)+Jij(2S-1)/4

as shown below.

In[47]:=
```
JA P[1,1/2,i,j,L]+ JB P[0,1/2,i,j,L] == (JA-JB) SdS[i,j,L]+
 (3JA+JB)/4*id[SdS[i,j,L]]//Normal//FullSimplify
(* for any JA=Jij(2S) and JB=Jij(2S-1)  *)
```

Out[47]=
```
True
```

This correspondence leads the definition of H^(1/2),

H^(1/2)=Σij (Jij(2S)-Jij(2S-1)) si·sj + E0,

E0=Σij (3Jij(2S)+Jij(2S-1)) /4,

which is written below Eq . (5) in the paper. Then, one can prove Eq.(S0) as

Hr ℂ = Σ Jij(s) Pij(s) ℂ = ℂ Σ [Jij(2S) pij(1) + Jij(2S-1) pij(0)] = ℂ Σ [( Jij(2S)-Jij(2S-1) )s_i · s_j + (3 Jij(2S)+Jij(2S-1)/4] = ℂ H^(1/2),

if one assumes Eqs.(S1)~(S3).

Let us consider the proof of Eqs.(S1)~(S3) for general L. A key is that projection operators Pij act as identity operators for the sites that are neither i nor j. Thus, it is enough to consider two-site systems as demonstrated below for S=3/2, redefining Eqs.(S1)~(S3) for two-site system.

In[48]:=
```
(* here, the default values i=1,j=2,L=2 are used. *)
S=3/2;
Eq[S1]:=(P[2S,S]+P[2S-2,S]) . ℂ[S]==ℂ[S] . P[1,1/2];
Eq[S2]:=P[2S-1,S] . ℂ[S]==ℂ[S] . P[0,1/2];
Eq[S3]:=Table[zeroMatrixQ[P[s,S] . ℂ[S]],{s,0,2S-3}];
And@@Flatten[{Eq[S1],Eq[S2],Eq[S3]}]
```

Out[52]=
```
True
```

For above two-site system, one can check spin-1/2 projection pij(s=1), pij(s=0), ℂ, Pij(2S), and so-on as shown below for S=3/2.

In[53]:=
```
P[1,1/2]//mf (* pij(s=1) for spin-1/2 *)
```

Out[53]//TraditionalForm=

$$\begin{pmatrix} 1 & 0 & 0 & 0 \\ 0 & \frac{1}{2} & \frac{1}{2} & 0 \\ 0 & \frac{1}{2} & \frac{1}{2} & 0 \\ 0 & 0 & 0 & 1 \end{pmatrix}$$

In[54]:=
```
P[0,1/2]//mf(*pij(s=0) for spin-1/2 *)
```

Out[54]//TraditionalForm=

$$\begin{pmatrix} 0 & 0 & 0 & 0 \\ 0 & \frac{1}{2} & -\frac{1}{2} & 0 \\ 0 & -\frac{1}{2} & \frac{1}{2} & 0 \\ 0 & 0 & 0 & 0 \end{pmatrix}$$

In[55]:=
```
ℂ[S]//mf (* (2S-1)^2 and 4 dim. ℂ for spin-S *)
```

Out[55]//TraditionalForm=

$$\begin{pmatrix} 1 & 0 & 0 & 0 \\ 0 & 1 & 0 & 0 \\ 0 & 0 & 0 & 0 \\ 0 & 0 & 0 & 0 \\ 0 & 0 & 1 & 0 \\ 0 & 0 & 0 & 1 \\ 0 & 0 & 0 & 0 \\ 0 & 0 & 0 & 0 \\ 0 & 0 & 0 & 0 \\ 0 & 0 & 0 & 0 \\ 0 & 0 & 0 & 0 \\ 0 & 0 & 0 & 0 \\ 0 & 0 & 0 & 0 \\ 0 & 0 & 0 & 0 \\ 0 & 0 & 0 & 0 \\ 0 & 0 & 0 & 0 \end{pmatrix}$$

In[56]:=
```
P[2S,S]//mf  (* Pij(s=2S) for spin-S *)
(* one can check P[2S-1,S], P[2S-2,S]... *)
```

Out[56]//TraditionalForm=

$$\begin{pmatrix}
1 & 0 & 0 & 0 & 0 & 0 & 0 & 0 & 0 & 0 & 0 & 0 & 0 & 0 & 0 & 0 \\
0 & \frac{1}{2} & 0 & 0 & \frac{1}{2} & 0 & 0 & 0 & 0 & 0 & 0 & 0 & 0 & 0 & 0 & 0 \\
0 & 0 & \frac{1}{5} & 0 & 0 & \frac{\sqrt{3}}{5} & 0 & 0 & \frac{1}{5} & 0 & 0 & 0 & 0 & 0 & 0 & 0 \\
0 & 0 & 0 & \frac{1}{20} & 0 & 0 & \frac{3}{20} & 0 & 0 & \frac{3}{20} & 0 & 0 & \frac{1}{20} & 0 & 0 & 0 \\
0 & \frac{1}{2} & 0 & 0 & \frac{1}{2} & 0 & 0 & 0 & 0 & 0 & 0 & 0 & 0 & 0 & 0 & 0 \\
0 & 0 & \frac{\sqrt{3}}{5} & 0 & 0 & \frac{3}{5} & 0 & 0 & \frac{\sqrt{3}}{5} & 0 & 0 & 0 & 0 & 0 & 0 & 0 \\
0 & 0 & 0 & \frac{3}{20} & 0 & 0 & \frac{9}{20} & 0 & 0 & \frac{9}{20} & 0 & 0 & \frac{3}{20} & 0 & 0 & 0 \\
0 & 0 & 0 & 0 & 0 & 0 & 0 & \frac{1}{5} & 0 & 0 & \frac{\sqrt{3}}{5} & 0 & 0 & \frac{1}{5} & 0 & 0 \\
0 & 0 & \frac{1}{5} & 0 & 0 & \frac{\sqrt{3}}{5} & 0 & 0 & \frac{1}{5} & 0 & 0 & 0 & 0 & 0 & 0 & 0 \\
0 & 0 & 0 & \frac{3}{20} & 0 & 0 & \frac{9}{20} & 0 & 0 & \frac{9}{20} & 0 & 0 & \frac{3}{20} & 0 & 0 & 0 \\
0 & 0 & 0 & 0 & 0 & 0 & 0 & \frac{\sqrt{3}}{5} & 0 & 0 & \frac{3}{5} & 0 & 0 & \frac{\sqrt{3}}{5} & 0 & 0 \\
0 & 0 & 0 & 0 & 0 & 0 & 0 & 0 & 0 & 0 & 0 & \frac{1}{2} & 0 & 0 & \frac{1}{2} & 0 \\
0 & 0 & 0 & \frac{1}{20} & 0 & 0 & \frac{3}{20} & 0 & 0 & \frac{3}{20} & 0 & 0 & \frac{1}{20} & 0 & 0 & 0 \\
0 & 0 & 0 & 0 & 0 & 0 & 0 & \frac{1}{5} & 0 & 0 & \frac{\sqrt{3}}{5} & 0 & 0 & \frac{1}{5} & 0 & 0 \\
0 & 0 & 0 & 0 & 0 & 0 & 0 & 0 & 0 & 0 & 0 & \frac{1}{2} & 0 & 0 & \frac{1}{2} & 0 \\
0 & 0 & 0 & 0 & 0 & 0 & 0 & 0 & 0 & 0 & 0 & 0 & 0 & 0 & 0 & 1
\end{pmatrix}$$

Above matrices are generated based on Eq.(4) in the paper. Using the matrices, one can prove matrix-relations Eqs.(S1)~(S3) for a  given S.  In next S .2 - 3, let us proceed to the proof for general S.

# S. 2 - 3 Proof for general S

Since Eqs.(S1)~(S3) for the two-site system have matrix-dimensions (2S+1)^2 and 4 for general spin-S, the proof is enough to consider (2S+1)^2-dimensional-vector equations for four states |ϕ〉=|↑〉|↑〉,|↑〉|↓〉,|↓〉|↑〉, and |↓〉|↓〉. For example, the matrix-equation [ Pij(2S) + Pij(2S-2) ] ℂ = ℂ pij(1) of Eq.(S1) becomes vector-equations

[ Pij(2S) + Pij(2S-2) ] ℂ |ϕ〉= ℂ pij(1)|ϕ〉

for the four states |ϕ〉, where pij(s) is spin-projection for spin-1/2. The four states |ϕ〉 are equivalent to spin-1/2 triplet |t_k〉 and singlet |s〉, defined as

|t_1〉=|↑〉|↑〉,
|t_0〉=(|↑〉|↓〉 + |↓〉|↑〉)/Sqrt[2],
|t_-1〉=|↓〉|↓〉,
|s_0〉=(|↑〉|↓〉 – |↓〉|↑〉)/Sqrt[2],

which is written in note[30]. The right hand sides of Eqs.(S1)~(S3) becomes

pij(1) |t_k〉 = |t_k〉, (S4)
pij(0) |t_k〉=0, (S5)
pij(1) |s_0〉 =0, (S6)
pij(0) |s_0〉= |s_0〉, (S7)

(k=-1,0,1). Eqs.(S4)~(S7) are valid due to the definition of spin-projection operator pij(s) as demonstrated below.

In[57]:=
```
ket2[m1_,m2_,s_:1/2]:=Flatten[KroneckerProduct[{ket[m1,s]},{ket[m2,s]}]];
t[1]:=ket2[+1/2,+1/2];
t[0]:=(ket2[+1/2,-1/2]+ket2[-1/2,+1/2])/Sqrt[2];
t[-1]:=ket2[-1/2,-1/2];
s[0]:=(ket2[+1/2,-1/2]-ket2[-1/2,+1/2])/Sqrt[2];
Eq[S4]:=P[1] . t[k]==1*t[k];
Eq[S5]:=P[0] . t[k]==0*t[k];
Eq[S6]:=P[1] . s[0]==0*s[0];
Eq[S7]:=P[0] . s[0]==1*s[0];
And@@Flatten[Join[Table[{Eq[S4],Eq[S5]},{k,-1,1}],{Eq[S6],Eq[S7]}]]
```

Out[66]=
```
True
```

The return value "True" means that Eqs.(S4)~(S7) are valid. Using Eqs.(S4)~(S7) to eliminate pij(s), the proof of Eqs.(S1)~(S3) is decomposed into the following six equations:

( Pij(2S)+Pij(2S-2) ) |T_k〉 =|T_k〉, (S8)
( Pij(2S)+Pij(2S-2) ) |S_0〉 =0, (S9)
Pij(2S-1) |T_k〉=0, (S10)
Pij(2S-1) |S_0〉= |S_0〉 , (S11)
Pij(s) |T_k〉 =0, (s<=2S-3) (S12)
Pij(s) |S_0〉= 0, (s<=2S-3) (S13)

(k=-1,0,1) , where the spin-S states are defined as

|T_k〉 = ℂ |t_k〉, |S_0〉= ℂ |s_0〉

as demonstrated for spin S=3/2.

In[67]:=
```
S=3/2;(* one can modify spin-S*)
Block[{s0,k},
T[k_]:=ℂ[S] . t[k];
𝒮[0]:=ℂ[S] . s[0];
Eq[S8]:=(P[2S,S]+P[2S-2,S]) . T[k]==1*T[k];
Eq[S9]:=(P[2S,S]+P[2S-2,S]) . 𝒮[0]==0*𝒮[0];
Eq[S10]:=P[2S-1,S] . T[k]==0*T[k];
Eq[S11]:=P[2S-1,S] . 𝒮[0]==1*𝒮[0];
Eq[S12]:=P[s0,S] . T[k]==0*T[k];
Eq[S13]:=P[s0,S] . 𝒮[0]==0*𝒮[0];
And@@Flatten[Join[Table[{Eq[S8],Eq[S10],Table[Eq[S12],{s0,0,2S-3}]},{k,-1,1}],
{Eq[S9],Eq[S11],Table[Eq[S13],{s0,0,2S-3}]}]]]
```

Out[67]= True

The return value "True" means that Eqs.(S8)~(S13) are valid for a given S=3/2.

Let us proceed the general S case. In general, following the textbooks, two spin-S system is spanned by |J,M⟩ with total spin J and its z-component M, (0<= J <= 2S, -J<= M <= J ). Let us consider the six states defined as

|J=2S,M=2S⟩ = |S⟩|S⟩,
|J=2S,M=2S-1⟩ = (|S⟩|S-1⟩ + |S-1⟩|S⟩)/Sqrt[2],
|J=2S,M=2S-2⟩ = (|S⟩|S-2⟩ + |S-2⟩|S⟩)/Sqrt[4+2/(2S-1)] + |S-1⟩|S-1⟩/Sqrt[2-1/(2S)],
|J=2S-1,M=2S-1⟩ = (|S⟩|S-1⟩ – |S-1⟩|S⟩)/Sqrt[2],
|J=2S-1,M=2S-2⟩ = (|S⟩|S-2⟩ – |S-2⟩|S⟩)/Sqrt[2] ,
|J=2S-1,M=2S-2⟩ = (|S⟩|S-2⟩ + |S-2⟩|S⟩)/Sqrt[4-1/S] – |S-1⟩|S-1⟩/Sqrt[4-(4S-3)/(2S-1)].

These basis |J,M⟩ are satisfying the equation

Pij(s) |J,M⟩ = δ_{s,J} |J,M⟩, (0<= s <=2S), (S14)

by definition of spin-projection Pij(s) as demonstrated for the six basis for S=3/2 below.

In[68]:=
```
Clear[JM]; (* JM[J,M], total spin J and z-component M *)
JM[2S,2S]:=ket2[S,S,S];
JM[2S,2S-1]:=(ket2[S,S-1,S]+ket2[S-1,S,S])/Sqrt[2];
JM[2S,2S-2]:=(ket2[S,S-2,S]+ket2[S-2,S,S])/Sqrt[4+2/(2S-1)]+
ket2[S-1,S-1,S]/Sqrt[2-1/(2S)];
JM[2S-1,2S-1]:=(ket2[S,S-1,S]-ket2[S-1,S,S])/Sqrt[2];
JM[2S-1,2S-2]:=(ket2[S,S-2,S]-ket2[S-2,S,S])/Sqrt[2];
JM[2S-2,2S-2]:=(ket2[S,S-2,S]+ket2[S-2,S,S])/Sqrt[4-1/S]-
ket2[S-1,S-1,S]/Sqrt[4-(4S-3)/(2S-1)];
Eq[S14]:=P[s,S] . JM[J,M]==KroneckerDelta[s,J]*JM[J,M];
And@@Flatten[Table[Eq[S14],{s,0,2S},{J,2S-2,2S},{M,2S-2,J}]]
```

Out[75]= True

Considering the definition of ℂ=Π |S⟩⟨↑|+|S-1⟩⟨↓|, one can show the relation

|T_1⟩=ℂ|t_1⟩ = ℂ |↑⟩|↑⟩ = |S⟩|S⟩=|J=2S,M=2S⟩,
|T_0⟩=ℂ|t_0⟩ = ℂ (|↑⟩| ↓⟩ + |↓⟩|↑⟩)/Sqrt[2] = (|S⟩|S-1⟩ + |S-1⟩|S⟩)/Sqrt[2] = |J=2S,M=2S-1⟩ ,
|S_0⟩=ℂ|s⟩ = ℂ (|↑⟩|↓⟩ – |↓⟩|↑⟩)/Sqrt[2] = (|S⟩|S-1⟩ – |S-1⟩|S⟩)/Sqrt[2] = |J=2S-1,M=2S-1⟩,

as demonstrated below.

In[76]:=
```
T[1]==JM[2S,2S]
```
Out[76]= True

In[77]:=
```
T[0]==JM[2S,2S-1]
```
Out[77]= True

In[78]:=
```
𝒮[0]==JM[2S-1,2S-1]
```
Out[78]= True

Using three equations above, one can prove Eqs.(S8)~(S13) directly via Eq.(S14), except for |t_-1⟩ . The remaining state |T_-1⟩ is written as a linear combination of |J=2S,M=2S-2⟩ and |J=2S-2,M=2S-2⟩ because

|T_-1⟩=ℂ|t_-1⟩ = ℂ |↓⟩|↓⟩ = |S-1⟩|S-1⟩

can be written as

|T_-1⟩= Sqrt[2S(2S-1)/(4S-1)^2] * (Sqrt[4+2/(2S-1)]|J=2S,M=2S-2⟩ - Sqrt[4-1/S] |J=2S-2,M=2S-2⟩ )

as demonstrated below.

In[79]:=
```
T[-1]==Sqrt[S (2S-1)/(4S-1)^2](Sqrt[4+2/(2S-1)]*JM[2S,2S-2]
-Sqrt[4-1/S]*JM[2S-2,2S-2])
```
Out[79]= True

Then, Eqs.(S8), (S10), (S12) have been proved also for |T_-1⟩ because of

(Pij(2S) + Pij(2S-2) ) ($\alpha$|J=2S,M=2S-2⟩ + $\beta$|J=2S-2,M=2S-2⟩ ) = $\alpha$|J=2S,M=2S-2⟩ + $\beta$|J=2S-2,M=2S-2⟩,

which comes from Eq.(S14). Here, one can understand why the condition Jij(2S)=Jij(2S-2) in Hr is required for the rigorous correspondence.

# S. 2 - 4 Summary

In summary, Eqs.(S8)~(S13) for general S, written in note[30] of the paper, have been proved in S.2-3. Based on Eqs.(S8)~(S13) for two-site system, one can prove Eqs.(S1)~(S3) for general L following S.2-2. Based on Eqs.(S1)~(S3) for general L and S, one can prove Eq.(S0) following S.2-2. Finally, Eq.(S0) leads the rigorous eigenstate correspondence.

As written in the paper, other degenerated states are given as |Ψs⟩ = (Stot^-)^s |Ψ0⟩ = (Stot^-)^s ℂ |$\psi$⟩ for any eigenstate |$\psi$⟩ of H^(1/2). After a spontaneous magnetization, the fractionally-magnetized state can written as |Ψ0⟩ if the spin-z axis is selected along with the magnetization.

In addition, any expectation value for the fractionally-magnetized ferromagnetic state |Ψ0⟩ of the spin-S model has a correspondence with that for |$\psi$⟩ of the spin-1/2 model, including correlation functions. Let us demonstrate calculation of correlation function ⟨sz_i, sz_j⟩ for L=8 and S=3/2. Here we calculate eigensystem ($\epsilon$,$\psi$) for spin 1/2 Heisenberg chain under the periodic boundary condition. Only four (nth=4) low energy states are calculated as follows.

In[80]:=
```
L=8;S=3/2;
defH[S,L];(* clear J, define Hr and Honehalf *)
(* Here we pbc Hamiltonian. You can use more traditional Hamiltonian. *)
J[i_,j_,2S]:=If[Mod[i-j,L,1]==1,1,0];
J[i_,j_,2S-1]:=0;
nth=4;(* one can modify *)
{ϵ,ψ}=Eigensystem[N[Honehalf],-nth];
Ψ0=Table[ℂ[S,L] . p,{p,ψ}];
ϵ
```

Out[85]=
```
{3.54126, 3.30037, 2.87158, 2.34891}
```

Since the eigen energy $\epsilon$ is descending order , one can obtain the ground state |$\psi$_nth⟩ with the lowest energy $\epsilon$_nth;

In[86]:=
```
ϵ⟦nth⟧ (* this might be the lowest energy in general *)
```

Out[86]=
```
2.34891
```

For the ground state |$\psi$_nth⟩, one can obtain correlation function ⟨sz_i, sz_j⟩ for i=1, and j=2,3,...,L as follows.

In[87]:=
```
corr[op_,i_,j_]:=op2[op,op,i,j,L];
sz[s_:1/2]:=Sop[s]⟦3⟧;
ave[op_,v_]:=ConjugateTranspose[v] . op . v/Norm[v];
Table[v[sz,1]×v[sz,j]==ave[corr[sz[],1,j],ψ⟦nth⟧],{j,2,L}]//Column
```

Out[90]=

$sz_1^{(1/2)}\, sz_2^{(1/2)} == -0.152129$

$sz_1^{(1/2)}\, sz_3^{(1/2)} == 0.0652593$

$sz_1^{(1/2)}\, sz_4^{(1/2)} == -0.0629843$

$sz_1^{(1/2)}\, sz_5^{(1/2)} == 0.0497077$

$sz_1^{(1/2)}\, sz_6^{(1/2)} == -0.0629843$

$sz_1^{(1/2)}\, sz_7^{(1/2)} == 0.0652593$

$sz_1^{(1/2)}\, sz_8^{(1/2)} == -0.152129$

For the corresponding eigenstate |Ψ0_nth⟩ in the spin-S system, one can obtain correlation function ⟨sz_i, sz_j⟩ for i=1, and j=2,3,...,L as follows.

In[91]:=
```
Table[v[sz,1,S]×v[sz,j,S]==ave[corr[sz[S],1,j],Ψ0⟦nth⟧],{j,2,L}]//Column
```

Out[91]=

$sz_1^{(3/2)}\, sz_2^{(3/2)} == 0.847871$

$sz_1^{(3/2)}\, sz_3^{(3/2)} == 1.06526$

$sz_1^{(3/2)}\, sz_4^{(3/2)} == 0.937016$

$sz_1^{(3/2)}\, sz_5^{(3/2)} == 1.04971$

$sz_1^{(3/2)}\, sz_6^{(3/2)} == 0.937016$

$sz_1^{(3/2)}\, sz_7^{(3/2)} == 1.06526$

$sz_1^{(3/2)}\, sz_8^{(3/2)} == 0.847871$

As shown above, the different values are obtained because the corresponding eigenstate |Ψ0_nth⟩ is partially magnetized. If one define new local spin-S operator

𝒮z = sz - (S-1/2)*Id,
where Id is identity matrix, then one can obtain the same results as follows.

In[92]:=
```
𝒮z[s_]:=sz[s]-(S-1/2)*id[sz[s]];
Table[v[𝒮z,1,S]×v[𝒮z,j,S]==ave[corr[𝒮z[S],1,j],Ψ0⟦nth⟧],{j,2,L}]//Column
```

Out[93]=

$\mathcal{S}z_1^{(3/2)}\ \mathcal{S}z_2^{(3/2)} == -0.152129$
$\mathcal{S}z_1^{(3/2)}\ \mathcal{S}z_3^{(3/2)} == 0.0652593$
$\mathcal{S}z_1^{(3/2)}\ \mathcal{S}z_4^{(3/2)} == -0.0629843$
$\mathcal{S}z_1^{(3/2)}\ \mathcal{S}z_5^{(3/2)} == 0.0497077$
$\mathcal{S}z_1^{(3/2)}\ \mathcal{S}z_6^{(3/2)} == -0.0629843$
$\mathcal{S}z_1^{(3/2)}\ \mathcal{S}z_7^{(3/2)} == 0.0652593$
$\mathcal{S}z_1^{(3/2)}\ \mathcal{S}z_8^{(3/2)} == -0.152129$

The agreement means the correspondence of expectation values after subtracting a ferromagnetic background of spin-(S-1/2) system (See Fig.2). Moreover, one can obtain the same entanglement entropy(EE) for bipartite subsystem with half system-size L/2 = 4 of the system-size L=8 as demonstrated below.

In[94]:=
```
ketL[j_,d_]:=SparseArray[{j,1}→1,{d,1}];
kp[j_,l1_,l2_,s_]:=KroneckerProduct[
SparseArray[{{i_,i_}→1},(2s+1)^l1],ketL[j,(2s+1)^l2]];
diad[m_]:=diad[m,m];
ρ[ψ_,La_,s_:1/2]:=Sum[diad[ψ . kp[j,La,L-La,s]],{j,1,(2s+1)^(L-La)}];
(* reduced density matrix ρ=Tr_{L-La}|ψ⟩⟨ψ| for system-size La *)
ee[x_]:=If[x==0,0,Chop[-x*Log[x]]];
EE[ρ_]:=Total[ee/@Eigenvalues[ρ]];
(* Entanglement entropy EE := Sum_n [- e_n*Log(e_n)] for
eigenvalues e_n of given reduced density matrix ρ*)
{v[EE,L/2]==EE[ρ[ψ⟦nth⟧,L/2]],v[EE,L/2,S]==EE[ρ[Ψ0⟦nth⟧,L/2,S]]}
```

Out[100]= $\{EE_4^{(1/2)} == 1.05117,\ EE_4^{(3/2)} == 1.05117\}$

For other degenerated |Ψs⟩ = (Stot^-)^s |Ψ0⟩, entanglement entropy can depends on s. The situation is same with the Ising-type fully-polarized ferromagnetic state |S,S,...,S⟩. The most important difference is quantum entanglement after the spontaneous magnetization; that is, |Ψ0⟩ has quantum entanglement while |S,S,...,S⟩ has no entanglement.

Finally, it should be emphasized that the corresponding state |Ψ0⟩ for spin-S system is just an exact eigenstate but not the ground state at this stage. To consider the ground state, numerical evidence is required as discussed in the paper. However, once |Ψ0⟩ is confirmed as the ground state, it is obvious that "ground states have quantum entanglement-reflecting corresponding spin-1/2 antiferromagnetic ground states in a ferromagnetic background".
